# Supplementary material for: Diffusion Policy: Visuomotor Policy Learning via Action Diffusion
Source: arXiv:2303.04137 source file (2024-03-14)
Supplement: Supplementary file 1 [file supp_main.tex]

\documentclass[conference]{IEEEtran}
\usepackage{times}
\usepackage[T1]{fontenc}
\usepackage[utf8]{inputenc}

% numbers option provides compact numerical references in the text. 
\usepackage[numbers]{natbib}
\usepackage{multicol}
\usepackage[pagebackref=true,breaklinks=true,bookmarks=true,colorlinks]{hyperref}
\input{format/packages}
\input{format/macros}

\pdfinfo{
   /Author (Homer Simpson)
   /Title  (Robots: Our new overlords)
   /CreationDate (D:20101201120000)
   /Subject (Robots)
   /Keywords (Robots;Overlords)
}

\begin{document}

% paper title
% \title{Diffusion Policy}
\title{Diffusion Policy \\ \LARGE{Supplemental Materials}}
%\title{Diffusion Policy: \\ \LARGE{Learning Visuomotor Policies with Conditional Diffusion Process}}
% You will get a Paper-ID when submitting a pdf file to the conference system
\author{Author Names Omitted for Anonymous Review. Paper-ID [6]}

%\maketitle

% \begin{figure*}[t]
%     \centering
%     \includegraphics[width=\linewidth]{figure/DP_teaser.pdf}
%     \caption{\textbf{Different Form of Policy Representations.} a) Explicit policy with different types of action representations.  b) Implicit policy learns an energy function conditioned on both action and observation and optimizes for actions that minimize the energy landscape c) Diffusion policy learns a gradient field to refine actions. \todo{update the figure with the same example. }  }
%     \label{fig:policy_rep}
%     %https://docs.google.com/drawings/d/1SNd5_khk3RsYuE9JCwUVjmRED-eF3UrO78XnzbOwE4Y/edit?usp=sharing
% \end{figure*}

\maketitle
\IEEEpeerreviewmaketitle

\input{text/supp.tex}

\bibliographystyle{plainnat}
\bibliography{references}

\end{document}
